# Supplementary material for: Clinical Utility of the Automatic Phenotype Annotation in Unstructured Clinical Notes: ICU Use Cases
Source: arXiv:2107.11665 source file (2021-11-24)
Supplement: Supplementary file 1 [file results_phenotyping_appendix.tex]

\begin{table}[!htbp]
\begin{subtable}[c]{1\textwidth}
\centering
\scalebox{0.80}{
\begin{tabular}{ |c|ccc|ccc| }
 \hline
 Method & \multicolumn{3}{|c|}{Exact Match} & \multicolumn{3}{|c|}{Generalised Match} \\
     & Precision  & Recall & F1 & Precision  &  Recall &  F1 \\
 \hline
Keyword & 0.7496 & 0.5223 & 0.6156 & 0.7883 & 0.6587 & 0.7177 \\
NCR & 0.7747 & 0.4851 & 0.5967 & 0.8778 & 0.5917 & 0.7069 \\ 
Clinphen & 0.8147 & 0.3148 & 0.4541 & 0.9337 & 0.4066 & 0.5665 \\
NCBO & \textbf{0.9186} & 0.3901 & 0.5477 & \textbf{0.9632} & 0.4711 & 0.6328 \\ 
cTAKES & 0.8250 & 0.3259 & 0.4673 & 0.9321 & 0.4287 & 0.5872 \\ 
MetaMap & 0.7909 & 0.4062 & 0.5367 & 0.8835 & 0.5384 & 0.6691 \\
MetaMapLite & 0.7968 & 0.4358 & 0.5634 & 0.8766 & 0.5720 & 0.6923 \\
MedCAT (Medmentions) & 0.7290 & 0.3321 & 0.4563 & 0.8305 & 0.4711 & 0.6012 \\
MedCAT (UMLS) & 0.8630 & 0.3889 & 0.5362 & 0.9311 & 0.5231 & 0.6699 \\
\hline
Ours (E) & 0.7334 & \textbf{0.5619} & \textbf{0.6363} & 0.7706 & 0.6972 & 0.7320 \\
Ours (E) w. Augmented Data & 0.7235 & 0.5556 & 0.6285 & 0.7741 & \textbf{0.6997} & \textbf{0.7351} \\ 
\hline
\end{tabular}}
\subcaption{Self-supervised setting.}
\end{subtable}

\bigskip
\begin{subtable}[c]{1\textwidth}
\centering
\scalebox{0.8}{
\begin{tabular}{ |c|ccc|ccc| }
 \hline
 Method & \multicolumn{3}{|c|}{Exact Match} & \multicolumn{3}{|c|}{Generalised Match} \\
     & Precision  & Recall & F1 & Precision  &  Recall &  F1 \\
 \hline
BERT            &   0.7132 & 0.5617 & 0.6285 & 0.8434 & 0.6844 & 0.7557  \\
BioBERT         &   0.6864 & 0.5728 & 0.6245 & 0.8335 & 0.7021 & 0.7622  \\
ClinicalBERT   &   0.6962 & 0.5630 & 0.6225 & 0.8429 & 0.6980 & 0.7637  \\
SciBERT         &   0.6898 & 0.5407 & 0.6062 & 0.8269 & 0.6671 & 0.7385  \\ \hline
Ours (E) w. Augmented Data  &   \textbf{0.7141} & \textbf{0.7123} & \textbf{0.7132} & \textbf{0.8463} & \textbf{0.8380} & \textbf{0.8421}  \\
\hline
\end{tabular}}
\subcaption{Fine-tuned setting.}
\end{subtable}

\caption{Results of phenotype annotation on the gold-standard test set in the self-supervised and fine-tuned setting respectively. NCR and ClinicalBERT overall achieve best F1 scores.}
\label{table:results_phenotyping_appendix}
\end{table}
